# Supplementary material for: Automated Machine Learning for Multi-Label Classification
Source: arXiv:2402.18198 source file (2024-02-28)
Supplement: Supplementary file 1 [file chapter-appendix.tex]

% !TEX root = ../my-thesis.tex
%
\chapter{Example Appendix}
\label{sec:appendix}
